# Supplementary material for: Brain Imaging Foundation Models, Are We There Yet? A Systematic Review of Foundation Models for Brain Imaging and Biomedical Research
Source: arXiv:2506.13306 source file (2025-06-16)
Supplement: Supplementary file 1 [file appendix.tex]

\appendix
\section{Example Appendix Section}
\label{app1}
